# Supplementary material for: PhysPart: Physically Plausible Part Completion for Interactable Objects
Source: arXiv:2408.13724 source file (2025-02-04)
Supplement: Supplementary file 1 [file 6-supplementary.tex]

\clearpage
\appendix
% \renewcommand\thefigure{A\arabic{figure}}
% \setcounter{figure}{0}
% \renewcommand\thetable{A\arabic{table}}
% \setcounter{table}{0}
% \renewcommand\theequation{A\arabic{equation}}
% \setcounter{equation}{0}
% \pagenumbering{arabic}% resets `page` counter to 1
% \renewcommand*{\thepage}{A\arabic{page}}
% \setcounter{footnote}{0}

\section{Implementation Details}
\label{appendix:implementation-details}

\subsection{Physical-Aware Losses and Metric}
\label{appendix:physical-plausibility-metric}

\textbf{Physical-Aware Losses.} We scale all parts to the unit cube with padding $0.2$ before transforming into SDF. For both physical-aware losses, we set the threshold $\alpha$ to $0.005$.

\textbf{Physical-Plausible Metric.} We detail the methodology of our proposed physical plausibility metric as follows. We first preprocess the meshes and discard those that are not watertight or have multiple large connected parts deemed physically infeasible. For the viable meshes, we employ a grid search with a grid length of $0.005$ around the part's ground truth position to identify all positions where both collision loss (\cref{eq:collision-loss}) and contact loss (\cref{eq:contact-loss}) fall below a predefined threshold of $\beta=0.04$. A part is then considered physically plausible if moving it along the $-z$ axis for a distance of $0.02$ (applicable to hinge doors) or along the $+x$ and $-x$ axes for a distance of $0.04$ (applicable to other part categories) results in the losses exceeding the threshold. Noe that the hyperparameters are chosen to ensure that more than 95\% of the ground truth meshes of each category are physically feasible. The pseudo-code for this algorithm is provided in \cref{algo:physical-plausible}.

\begin{algorithm}[t]
\SetKwInOut{Input}{input}\SetKwInOut{Output}{output}\SetKw{Return}{return}\SetKwInOut{Initiate}{initiate}\SetKw{False}{false}\SetKw{True}{true}\SetKw{And}{and}\SetKw{Exists}{exists}\SetKw{Where}{where}\SetKw{Or}{or}
    \Input{Object's point cloud $\mathcal{P}$, predicted missing part's mesh $x$, set of position candidate $C_1$ determined by grid search, set of small movement $C_2$, and loss margin $\beta$.}
    \Output{Whether the predicted mesh $x$ is physically plausible}
    \Initiate{$C_0=\emptyset$}
    \BlankLine
    Remove components in $x$ with volume $< 10^{-7}$ \;
    \If{$x$ \text{contains multiple components or is not watertight}}{
    \Return \False\;
    }
    Transform the mesh $x$ into SDF representation $X$\;
     \ForAll{position candidate $c \in C_1$}{
        $P^c \leftarrow P-c$;~~\tcp{translate point cloud by $-c$}
        \If{$\ell_{collision-m}(X,P^{c})<\beta$ \And $\ell_{contact-m}(X,P^{c})<\beta$
        }{Add $c$ to $C_0$\;}
    }
    \ForAll{$c' \in C_2$}{\If{\Exists $c \in C_0$ \Where ($\ell_{collision-m}(X,P^{c+c'})\geq\beta$ \Or $\ell_{contact-m}(X,P^{c+c'})\geq\beta$)}{\Return \True\;}}
    \Return \False\;
     
    \caption{Physical Plausibility Metric}
    \label{algo:physical-plausible}
\end{algorithm}

\subsection{Experimental Configuration}

\textbf{Pose Proposal Module.} The Pose Proposal Module is trained separately for each part category. We train for 100 epochs on a single NVIDIA RTX 4090 with batch size 8. We adopt the Adam optimizer and a $10^{-4}$ learning rate. The architecture is the same as GenPose~\cite{zhang2023genpose}.

\textbf{3D Vector Quantizer.} The 3D-VQVAE model is trained using all part instances from the GAPartNet~\cite{geng2022gapartnet} dataset and is shared across all part categories. We train the model for 150000 iterations on 8 NVIDIA V100 GPUs with batch size 1. We adopt the Adam optimizer and cosine learning rate scheduler with base learning rate $10^{-5}$. Detailed architecture is shown in \cref{fig:architecture}.

\textbf{Part Generation Module.} The part generation diffusion module is trained separately for each part category. We train the model for 100000 iterations on 8 NVIDIA V100 GPUs with batch size 4. We adopt the Adam optimizer and cosine learning rate scheduler with base learning rate $10^{-5}$. Guidance weights are set to $\omega_1=3$ and $\omega_2=1$ during loss-guided sampling. \cref{fig:architecture} illustrates the details.

\textbf{Part Manipulation Interaction Policy. } 
(1) Slider Drawer: To retrieve items from an open drawer, the gripper moves along the z-axis. To open a drawer, it approaches along the x-axis, typically aiming to grasp a handle on the drawer's front face.
(2) Hinge Door: For hinge doors with front-facing handles, the gripper grabs the handle to open the door. After grasping the handle, it rotates around the predicted hinge axis to complete the opening or closing action. For doors without handles, if the door is ajar, the gripper clamps the outer edge along the y-axis of the bounding box to open it.
(3) Hinge Knob: For hinge knobs, the gripper clamps the knob like a round handle and rotates the end-effector to perform the task.
(4) Fixed Handle: The interaction policy for linear fixed handles mirrors that of round fixed handles. The gripper’s opening direction should be perpendicular to the linear fixed handle, aligning parallel to the y-axis of the predicted bounding box.

\textbf{Part Manipulation Interaction Experiments. }
We employ a heuristic-based interaction policy to open drawers and doors, manipulate handles, and rotate knobs. Once we determine the part pose, our policy immediately provides the corresponding grasping pose. We then use cuRobo \cite{sundaralingam2023curobo} to position our gripper at the grasping pose. Following this, our interaction policy and predicted axis guide the design of the end-effector trajectory to match the part’s movement trajectory, interpolating it with a time step of $\frac{1}{200}$. Using Inverse Kinematics and a PID controller, we compute joint poses and maneuver the end-effector along the defined trajectory. Our implementation is independent of ROS, ensuring compatibility with various simulators.

\begin{figure}[t]
    \centering
    \includegraphics[width=\linewidth]{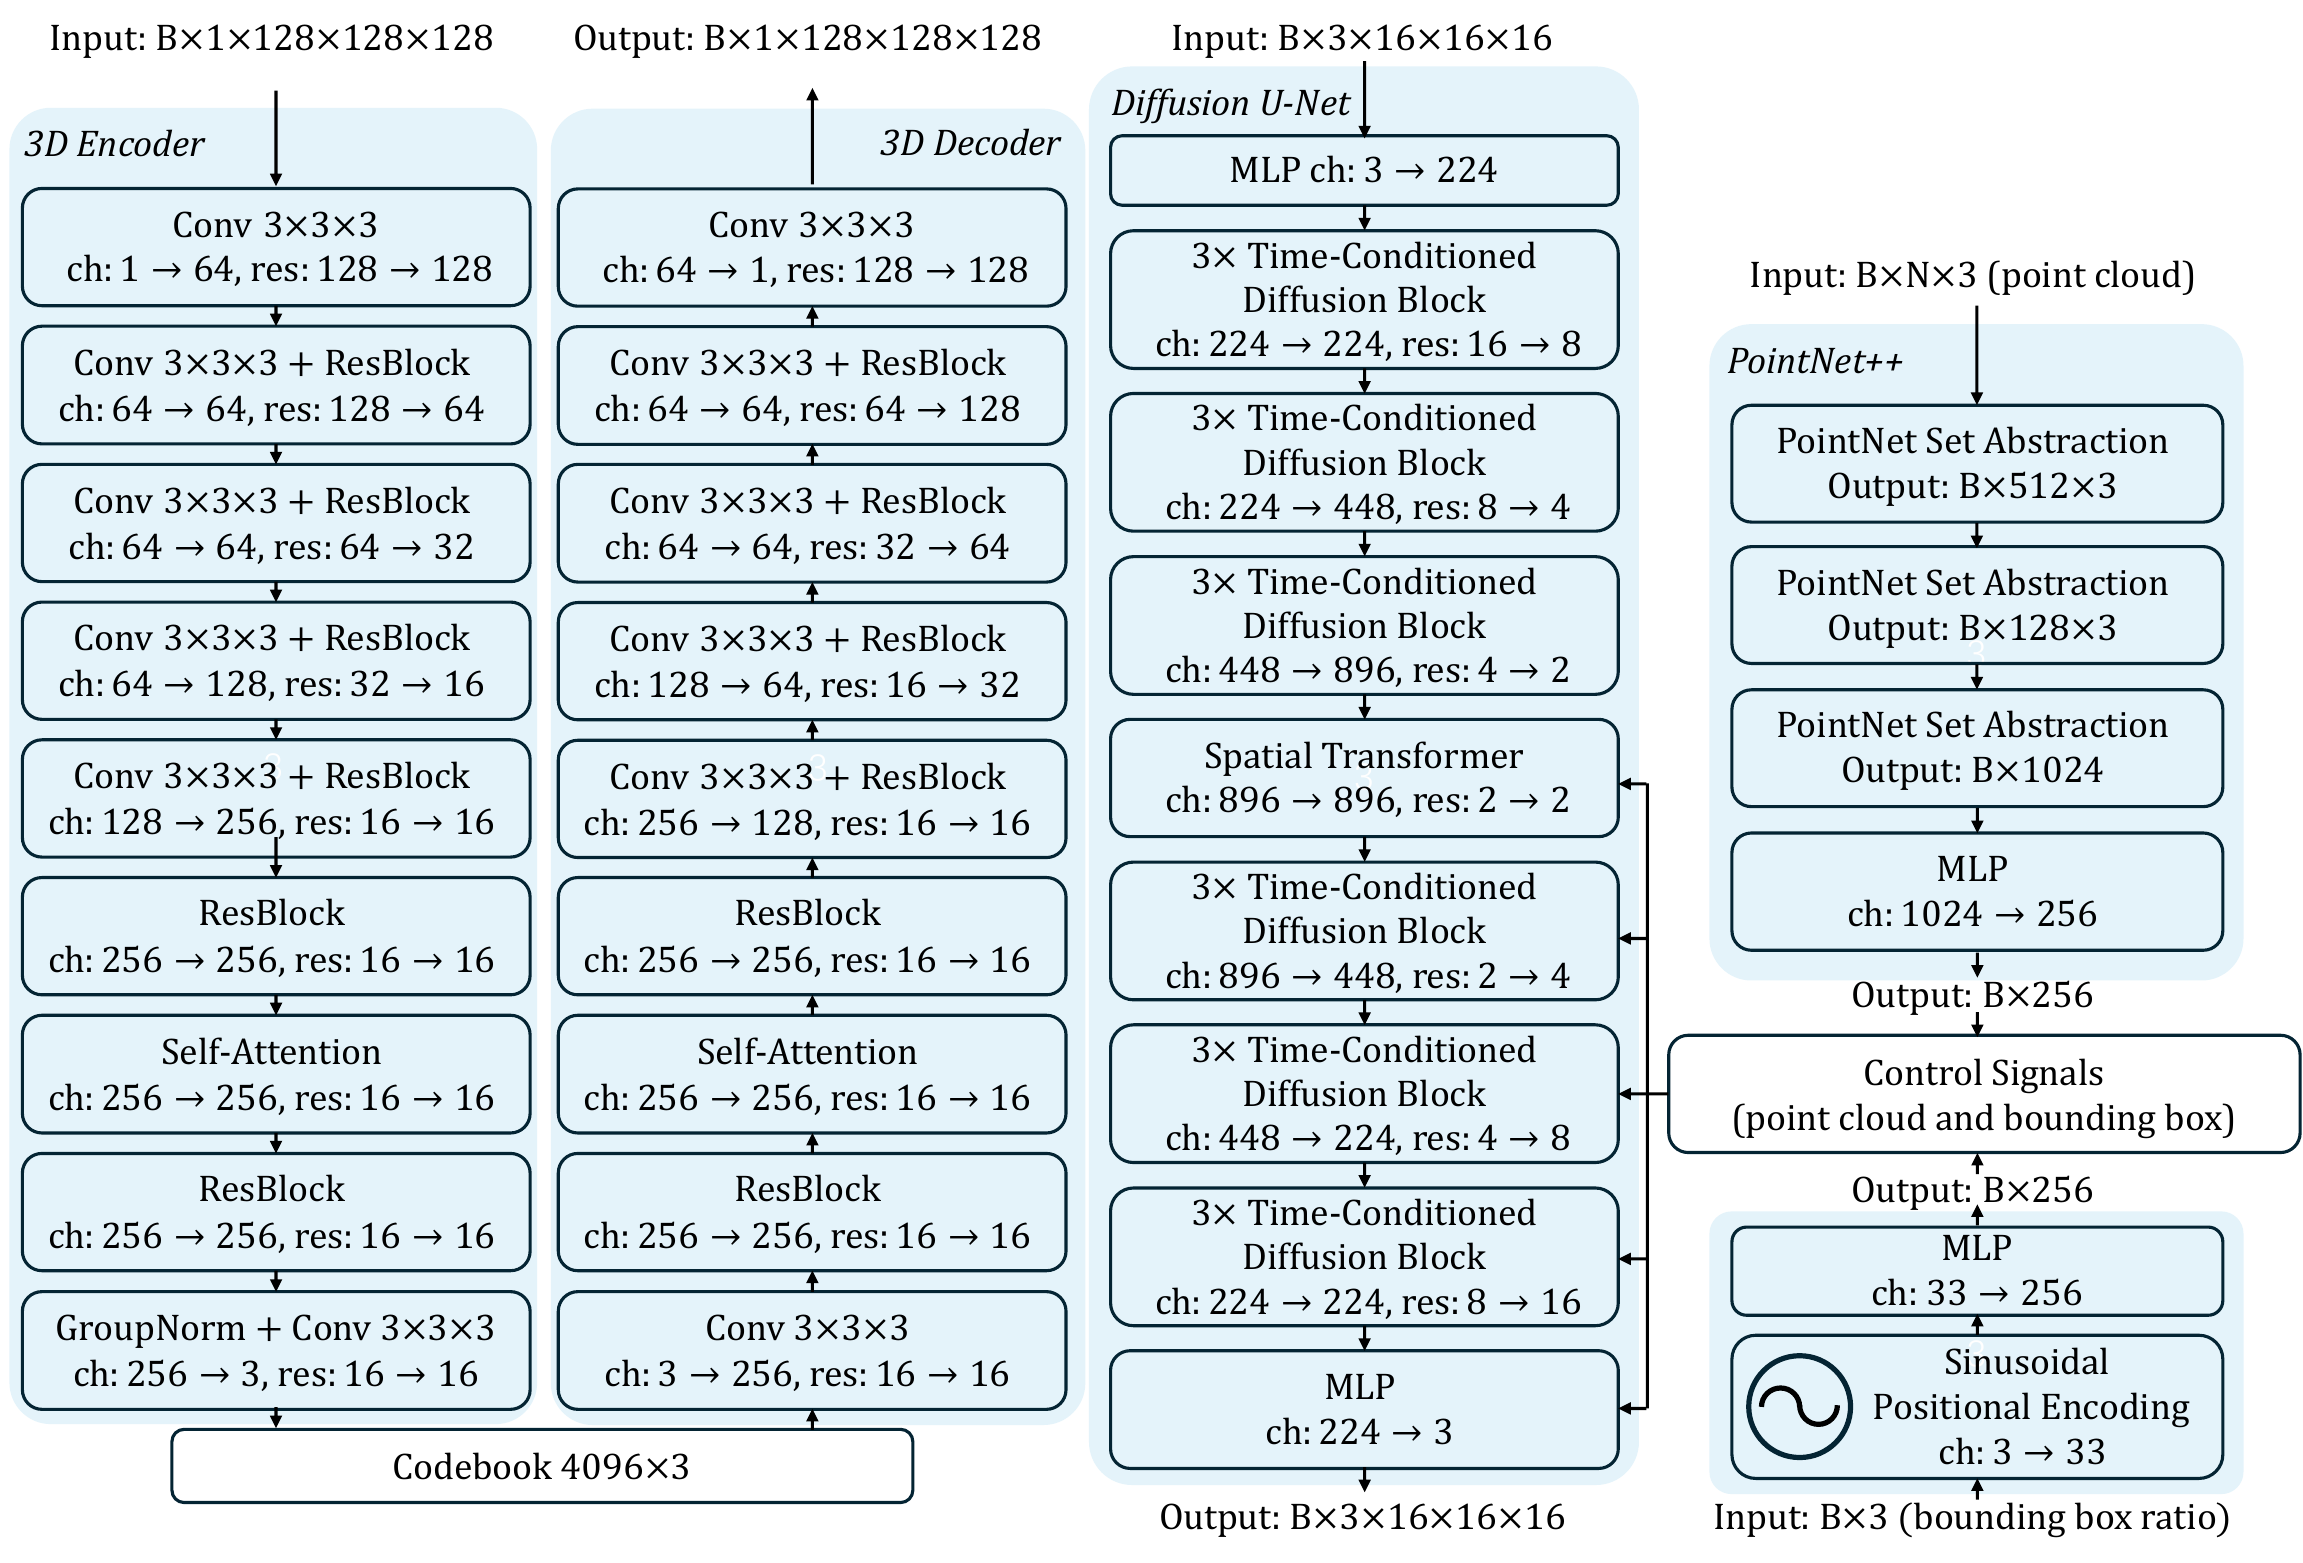}
    \caption{Architecture of our proposed physically plausible generation framework.}
    \label{fig:architecture}
\end{figure}

\section{Additional Experiments}
\label{appendix:additional-experiments}

\subsection{Additional Quantitative Results}
\label{appendix:additional-quantitative}

\myparagraph{Ablation studies on generating dependent parts.} \cref{tab:ablation-dependent} presents ablation studies on dependent parts generation to further validate our design choice to incorporate bounding box conditions into the diffusion model and employ a diffusion-based architecture for pose prediction. Similar to the results for generating self-moving parts shown in \cref{tab:ablation-self-moving}, the inclusion of both designs consistently yields superior results, further justifying the effectiveness of our approach in physical-plausible generation.

\begin{table}[t]
    \small
    \centering
    \caption{Ablation studies on the pose proposal module and the conditional generation module for~\textit{dependent} parts.}
    \vspace{1mm}
     \begin{tabular}{l |  C{37pt} C{36pt} C{36pt} | C{36pt} C{36pt} C{36pt}}
    \toprule
      \multirow{2}{*}{Method} & \multicolumn{3}{c|}{Line handle} & \multicolumn{3}{c}{Hinge knob}  \\
      & CD~$\downarrow$ & F-score $\uparrow$ & Phys.~(\%) & CD $\downarrow$ & F-score $\uparrow$  & Phys.~(\%) \\ \midrule
      Regress. pose proposal & 0.00252 & 0.655 & 74.2 & 0.00036 & 0.847 & 81.1 \\ \midrule
      w/o bbox condition & 0.00784 & 0.572 & 67.0 & 0.00033 & 0.885 & 80.7  \\ \midrule
      Full version & \textbf{0.00173} & \textbf{0.744} & \textbf{85.9} & \textbf{0.00024} & \textbf{0.917} & \textbf{84.2} \\
      \bottomrule
    \end{tabular}
    \label{tab:ablation-dependent}
\end{table}

\subsection{Additional Qualitative Results}

\textbf{Single Part Generation.} We present additional single part generation results in \cref{fig:appendix-part-gen-1,fig:appendix-part-gen-2}. While the baseline method frequently struggles to generate parts that meet physical constraints, our approach consistently yields high-fidelity part-generation results.

\begin{figure}[t]
    \centering
    \includegraphics[width=\linewidth]{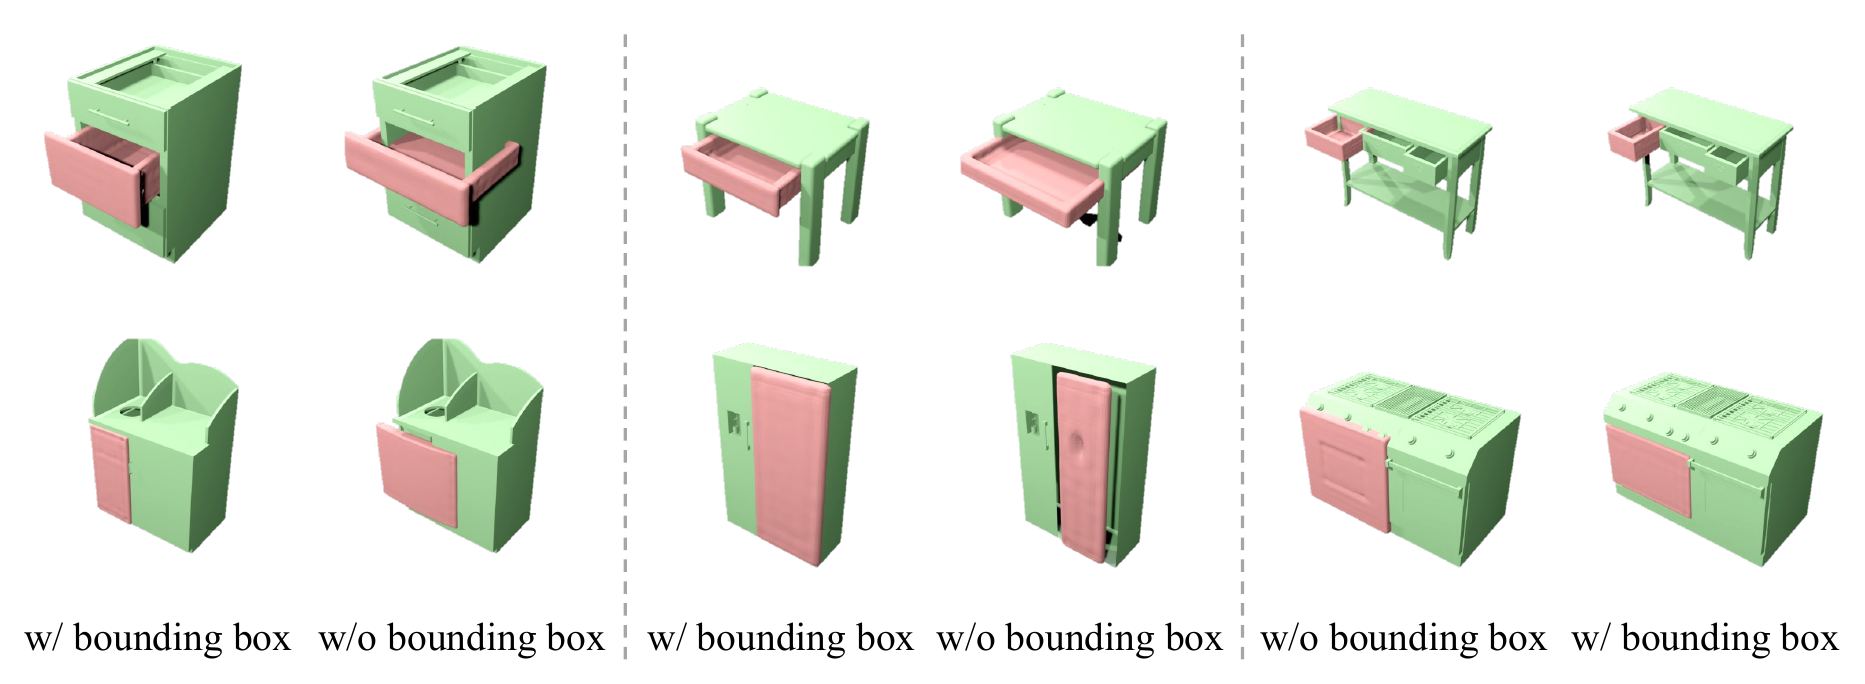}
    \vspace{-2mm}
    \caption{\textbf{Comparison between whether or not using the bounding box as an additional condition.} Incorporating the bounding box beside the point cloud enhances the fit of the generated part to the given object.}
    \label{fig:ablation-bbox}
\end{figure}

\begin{figure}
    \centering
    \includegraphics[width=\linewidth]{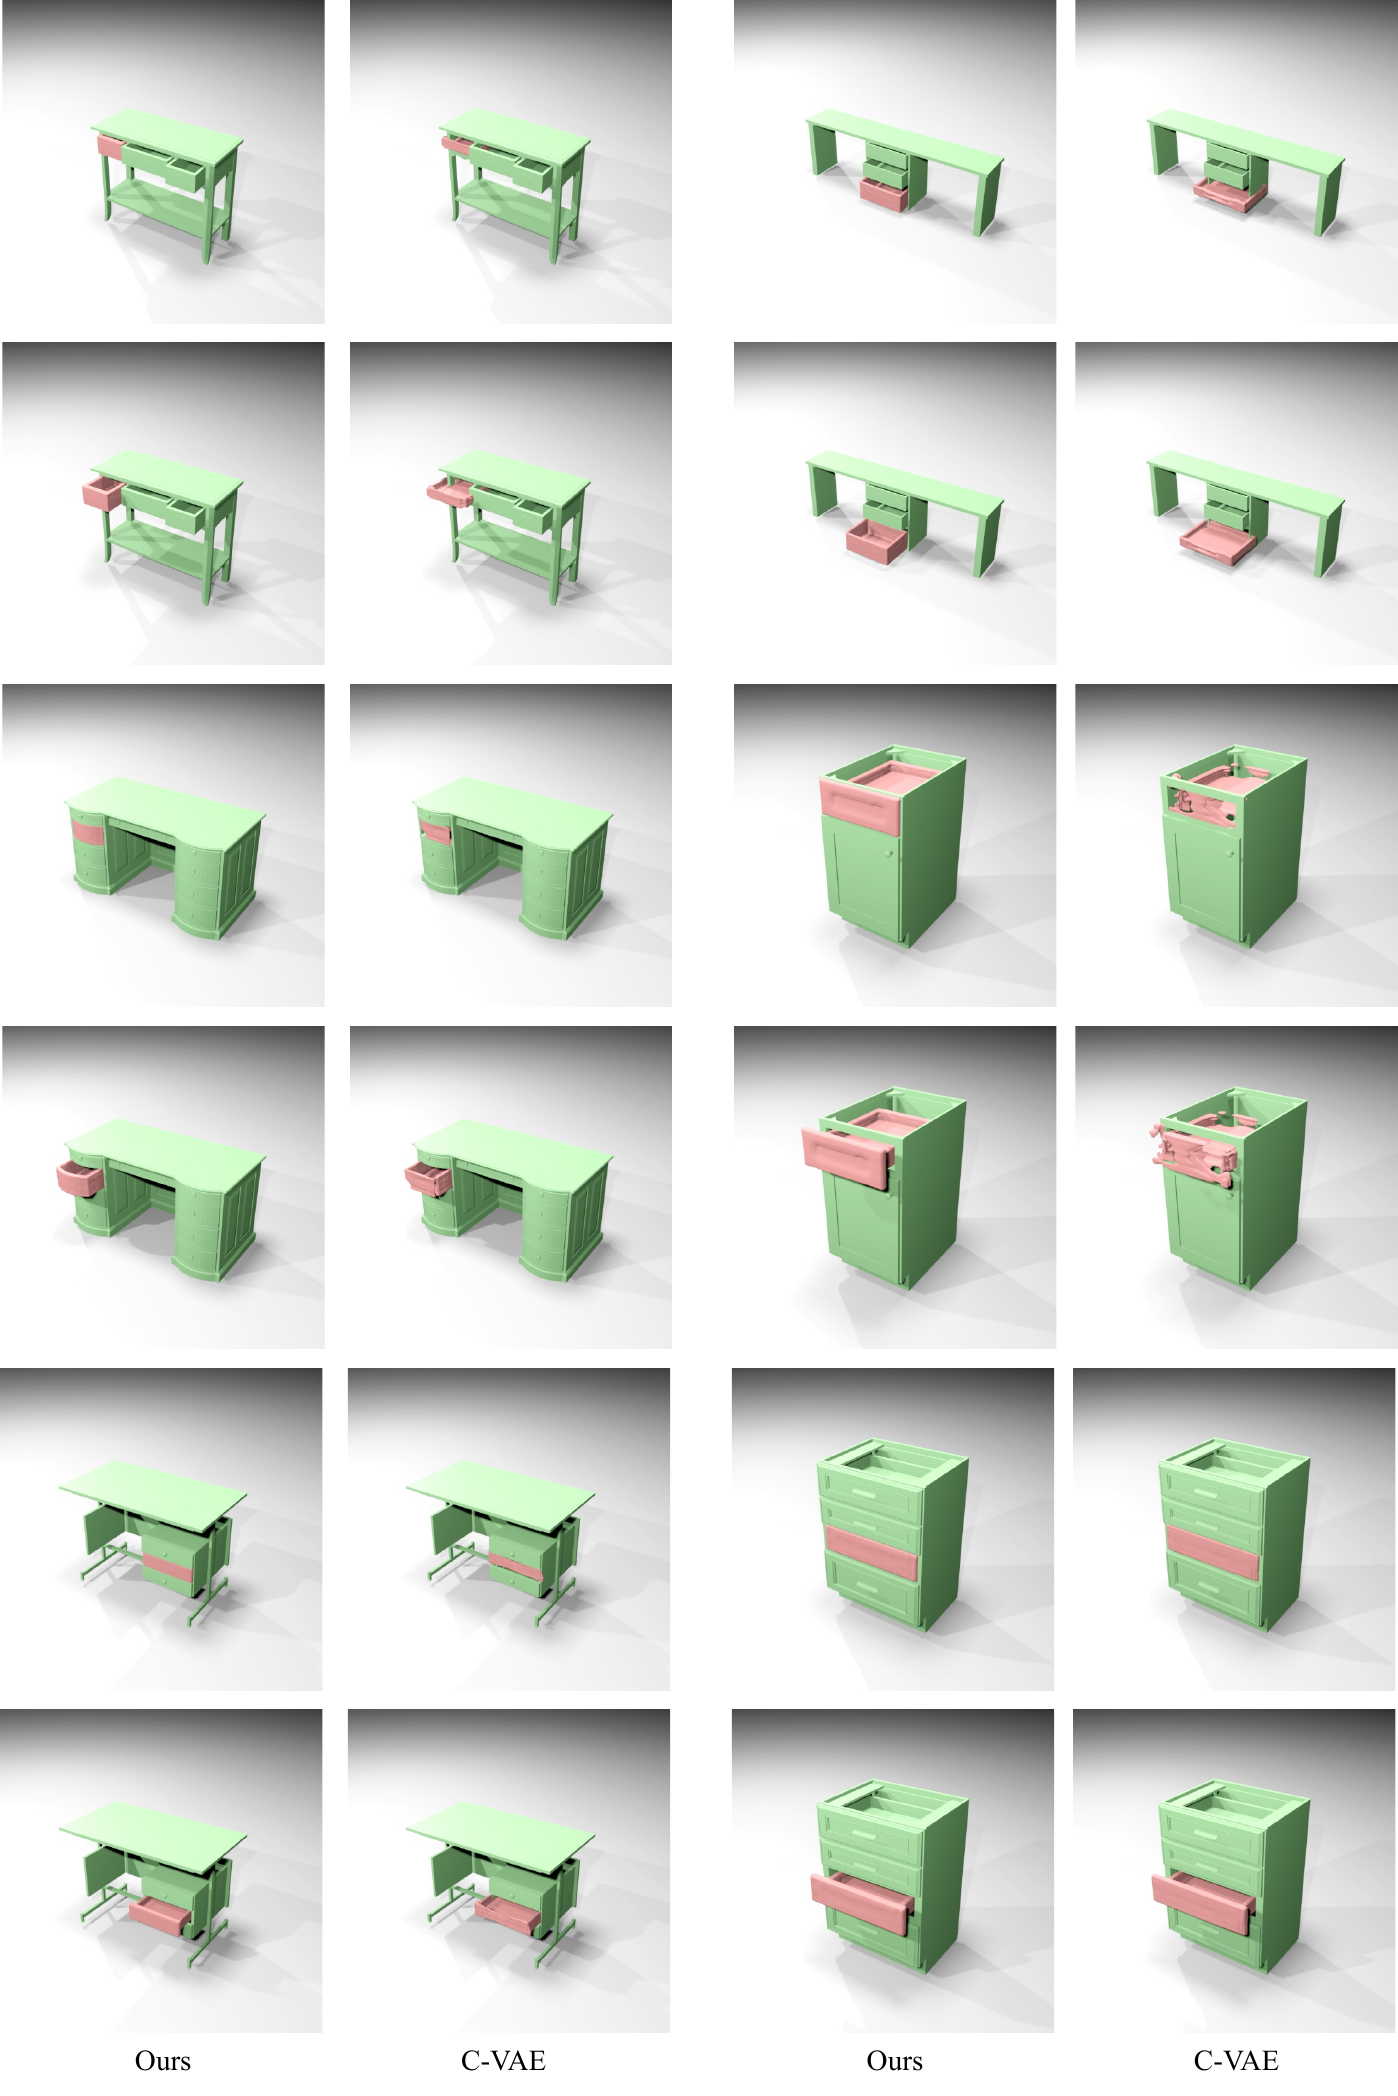}
    \caption{Qualitative single part generation results.}
    \label{fig:appendix-part-gen-1}
\end{figure}

\begin{figure}
    \centering
    \includegraphics[width=\linewidth]{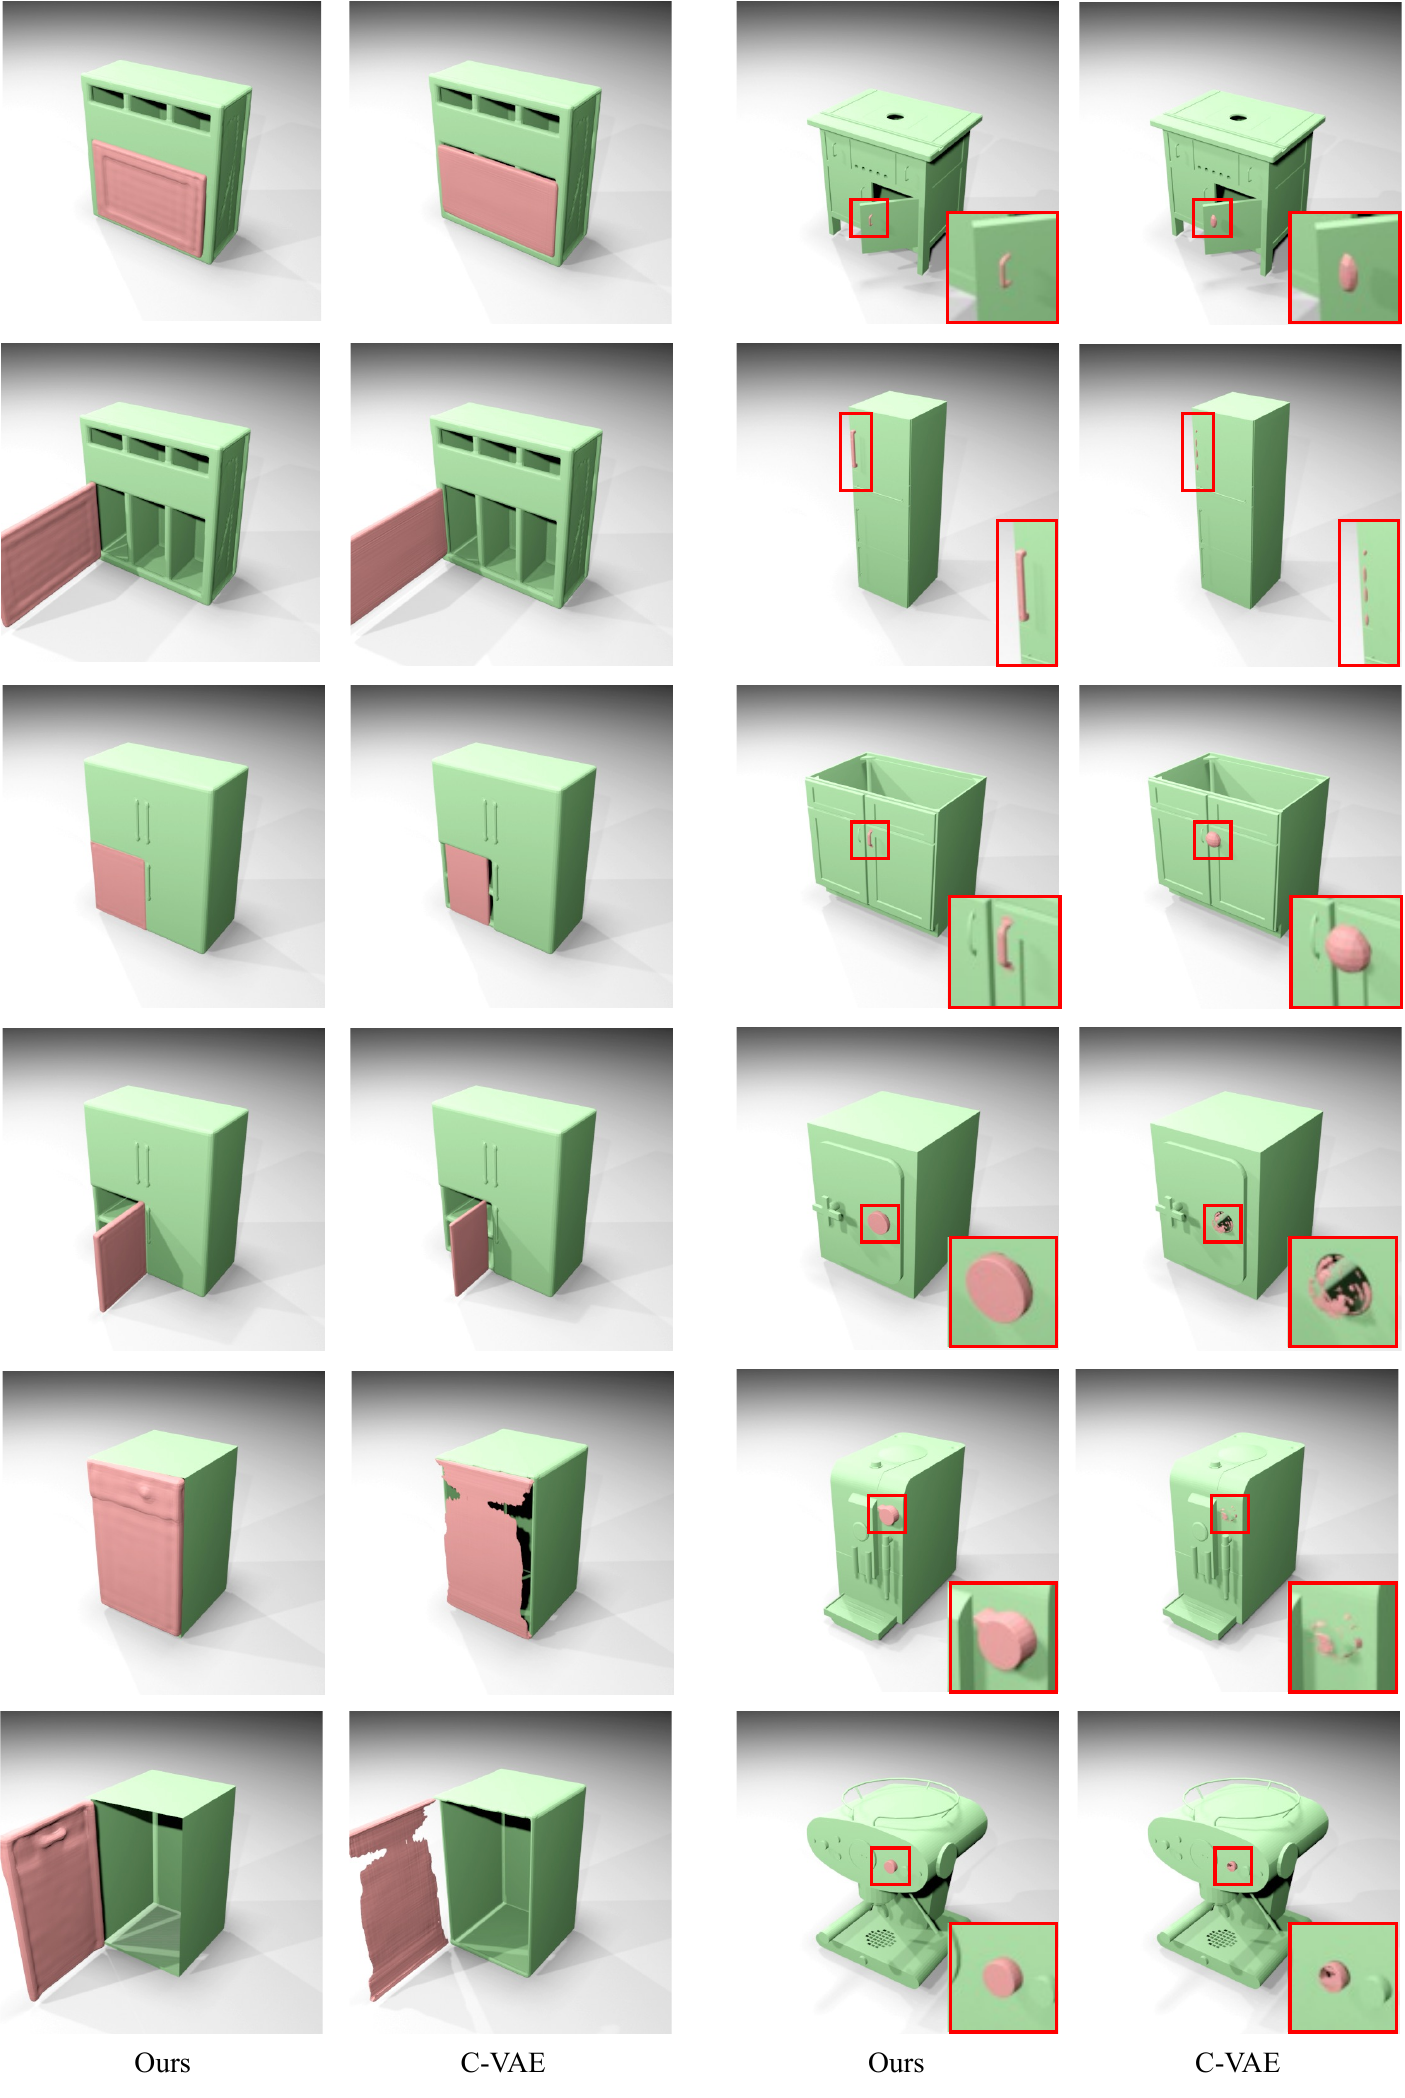}
    \caption{Qualitative single part generation results.}
    \label{fig:appendix-part-gen-2}
\end{figure}
